# Supplementary material for: QuadrupedGPT: Towards a Versatile Quadruped Agent in Open-ended Worlds
Source: arXiv:2406.16578 source file (2024-12-03)
Supplement: Supplementary file 1 [file para_range_bak.tex]

% Please add the following required packages to your document preamble:
% \usepackage{multirow}
\begin{table}[htb]
\centering
\caption{Location ranges for adjustable parameters.}
\label{tab: para_range}
\begin{tabular}{llc}
\toprule
                                         & \multicolumn{2}{c}{LOCATION RANGE} \\
\midrule
\multirow{5}{*}{Body Height (m)}         & Very High      & 0.4$\sim$0.45     \\
                                         & High           & 0.3$\sim$0.4      \\
                                         & Medium         & 0.2$\sim$0.3      \\
                                         & Low            & 0.15$\sim$0.2     \\
                                         & Very Low       & 0.1$\sim$0.15     \\
\midrule
\multirow{5}{*}{Stepping Frequency (Hz)} & Very High      & 3.5$\sim$4        \\
                                         & High           & 3$\sim$3.5        \\
                                         & Medium         & 2.5$\sim$3        \\
                                         & Low            & 2$\sim$2.5        \\
                                         & Very Low       & 1.5$\sim$2        \\
\midrule
\multirow{5}{*}{Foot Swing Height (m)}   & Very High      & 0.21$\sim$0.25    \\
                                         & High           & 0.16$\sim$0.21    \\
                                         & Medium         & 0.11$\sim$0.16    \\
                                         & Low            & 0.07$\sim$0.11    \\
                                         & Very Low       & 0.03$\sim$0.07    \\
\midrule
\multirow{5}{*}{Body Pitch (rad)}        & Very Positive  & 0.24$\sim$0.4     \\
                                         & Positive       & 0.08$\sim$0.24    \\
                                         & Neural         & -0.08$\sim$0.08   \\
                                         & Negative       & -0.24$\sim$-0.08  \\
                                         & Very Negative  & -0.4$\sim$-0.24   \\
\midrule
\multirow{5}{*}{Foot Stance Width (m)}   & Very High      & 0.37$\sim$0.45    \\
                                         & High           & 0.29$\sim$0.37    \\
                                         & Medium         & 0.21$\sim$0.29    \\
                                         & Low            & 0.13$\sim$0.21    \\
                                         & Very Low       & 0.05$\sim$0.13    \\
\midrule
\multirow{4}{*}{Gait Type ($\theta$)}    & Pronking       & $[0, 0, 0]$       \\
                                         & Trotting       & $[0.5, 0, 0]$     \\
                                         & Bounding       & $[0, 0.5, 0]$     \\
                                         & Pacing         & $[0, 0, 0.5]$    \\
\bottomrule
\end{tabular}
\end{table}
